# Supplementary material for: ActPlan-1K: Benchmarking the Procedural Planning Ability of Visual Language Models in Household Activities
Source: arXiv:2410.03907 source file (2024-10-04)
Supplement: Supplementary file 1 [file supplement.tex]

Hallucinations, one of the evident problems existing in generative language models from early GPT to recent GPT4, in which the models tend to produce content that is nonsensical or untruthful in relation to certain sources. 

Large LLMs are still lack of domain knowledge (e.g., commonsense). To alleviate the error in applying LLMs for solving commonsense related tasks, we propose to instruct tuning the models with commonsense knowledge generated from CSKGs, which is of low cost and high generalizability across various commonsense related tasks. Our method is data efficient compared to VERA. 

symbolic logic and natural language logic.
We propose a new benchmark to evaluate the logic reasoning ability of LLMs. Intuition is that rule mining or reasoning over knowledge graph, reasoning with natural language from LLM. To help LLM think rigorously like the logic over knowledge graph.

Logic-LLM. LLM+symbolic solver.

Complex logical reasoning in low-dimensional embedding space. logical queries/complex queries.
Complex logical query. EFOL. complex query embedding to model the quantification, conjunction, disjunction, and negation operators, as well as entity and relation embedding (GQE, Query2Box, and BetaE, GNNQE). Fuzzy logic (FuzzQE). t-norms and t-conorms. fuzzy conjunction, disjunction, and negation. 

RDF, proposition logic. explanation graph. Current explanation graph is based on entailment for reasoning chain. What is the relation between entailment and logic operations on KG? Structured reasoning over \textbf{commonsense or eventuality knowledge graph} with natural language. LLMs are good at solving QA form tasks. Are LLMs able to solve logical tasks with complicated logic?
